# Supplementary material for: IdeaBench: Benchmarking Large Language Models for Research Idea Generation
Source: arXiv:2411.02429 source file (2024-10-31)
Supplement: Supplementary file 2 [file checklist.pdf]

This paper:

- Includes a conceptual outline and/or pseudocode description of AI methods introduced YES
- Clearly delineates statements that are opinions, hypothesis, and speculation from objective facts and results YES
- Provides well marked pedagogical references for less-familiare readers to gain background necessary to replicate the paper YES

Does this paper make theoretical contributions? NO

If yes, please complete the list below.

- All assumptions and restrictions are stated clearly and formally. (yes/partial/no)
- All novel claims are stated formally (e.g., in theorem statements). (yes/partial/no)
- Proofs of all novel claims are included. (yes/partial/no)
- Proof sketches or intuitions are given for complex and/or novel results. (yes/partial/no)
- Appropriate citations to theoretical tools used are given. (yes/partial/no)
- All theoretical claims are demonstrated empirically to hold. (yes/partial/no/NA)
- All experimental code used to eliminate or disprove claims is included. (yes/no/NA)

Does this paper rely on one or more datasets? YES

If yes, please complete the list below.

- A motivation is given for why the experiments are conducted on the selected datasets YES
- All novel datasets introduced in this paper are included in a data appendix. YES
- All novel datasets introduced in this paper will be made publicly available upon publication of the paper with a license that allows free usage for research purposes. YES
- All datasets drawn from the existing literature (potentially including authors' own previously published work) are accompanied by appropriate citations. NA
- All datasets drawn from the existing literature (potentially including authors' own previously published work) are publicly available. NA
- All datasets that are not publicly available are described in detail, with explanation why publicly available alternatives are not scientifically satisfying. NA

Does this paper include computational experiments? YES

If yes, please complete the list below.

- Any code required for pre-processing data is included in the appendix. YES
- All source code required for conducting and analyzing the experiments is included in a code appendix. YES

- All source code required for conducting and analyzing the experiments will be made publicly available upon publication of the paper with a license that allows free usage for research purposes. YES
- All source code implementing new methods have comments detailing the implementation, with references to the paper where each step comes from YES
- If an algorithm depends on randomness, then the method used for setting seeds is described in a way sufficient to allow replication of results. NA
- This paper specifies the computing infrastructure used for running experiments (hardware and software), including GPU/CPU models; amount of memory; operating system; names and versions of relevant software libraries and frameworks. YES
- This paper formally describes evaluation metrics used and explains the motivation for choosing these metrics. YES
- This paper states the number of algorithm runs used to compute each reported result. NO
- Analysis of experiments goes beyond single-dimensional summaries of performance (e.g., average; median) to include measures of variation, confidence, or other distributional information. NO
- The significance of any improvement or decrease in performance is judged using appropriate statistical tests (e.g., Wilcoxon signed-rank). NO
- This paper lists all final (hyper-)parameters used for each model/algorithm in the paper's experiments. YES
- This paper states the number and range of values tried per (hyper-) parameter during development of the paper, along with the criterion used for selecting the final parameter setting. NA
